# Supplementary material for: Improving Energy Saving of One-sided Matrix Decompositions on CPU-GPU Heterogeneous Systems
Source: arXiv:2301.03166 source file (2023-04-26)
Supplement: Supplementary file 1 [file appendix.tex]

\appendix
\section{Artifact Appendix}
\subsection{Abstract}
This artifact contains the software framework (PowerLA) for energy saving matrix decomposition evaluation. It includes the energy-saving implementations of Cholesky, LU, and QR decomposition using H2R, SR, and BSR approaches. The framework is built based on the hybrid matrix decomposition algorithms in the MAGMA library. This artifact is available at: \href{https://doi.org/10.5281/zenodo.7317070}{https://doi.org/10.5281/zenodo.7317070}

\subsection{Hardware requirements}

\begin{itemize}
\item
  x86 CPU and NVIDIA GPUs (tested on a server with Intel Core i7-9700K
  with NVIDIA RTX 2080 Ti)
\end{itemize}

\subsection{OS requirements}
\begin{itemize}
\item
  Linux operating system (tested on Ubuntu 18.04)
\end{itemize}

\subsection{Software dependencies/configurations}
\begin{itemize}
\item For measuring CPU power:
  \href{https://github.com/sosy-lab/cpu-energy-meter}{cpu-energy-meter}
\item For adjusting CPU clock frequency: \href{https://wiki.archlinux.org/title/CPU_frequency_scaling}{cpupower}
\item For adjusting CPU core voltage:
  \href{https://wiki.archlinux.org/title/Undervolting\_CPU}{intel-undervolt}
\item For running GPU code: CUDA 11.4+.
\item For measuring GPU power, control GPU clock offset: NVIDIA GPU driver 450.80.02+.
\item For enabling GPU overclocking, set \href{https://wiki.archlinux.org/title/NVIDIA/Tips\_and\_tricks}{Coolbits} to the maximum allowed.
  The Coolbits on the tested system was set to \texttt{28}.
\item For compilation: GCC 7.5.0+ and NVCC 11.4+.
\item For configuring the project: CMake 2.8+.
\end{itemize}

\subsection{Building our PowerLA
framework}

\begin{itemize}
\item
  The PowerLA framework was built based on the MAGMA library v 2.5.4, so
  it uses the same build system as the MAGMA library. Please follow the
  \texttt{README.md} in the root directory to build PowerLA.
\end{itemize}

\subsection{Running optimized matrix
decompositions}
1. The major three one-sided matrix decomposition
algorithms (Cholesky, LU, and QR) are optimized. They are implemented
in:

\begin{itemize}
\item
  Cholesky: ./src/dportf\_gpu.cpp; ./src/sportf\_gpu.cpp
\item
  LU: ./src/dgetrf\_gpu.cpp; ./src/sgetrf\_gpu.cpp
\item
  QR: ./src/dgeqrf\_gpu.cpp; ./src/sgeqrf\_gpu.cpp
\end{itemize}

In each source code file, we added the following variables to control
the energy-saving and fault-tolerance behavior of each matrix
decomposition.

\begin{itemize}
\item
  \texttt{int\ tmu\_curr\_freq} and \texttt{int\ tmu\_base\_freq}: set
  the current and based clock frequency of GPU. They should be the same.
\item
  \texttt{int\ tmu\_base\_offset}: set the base clock offset of GPU.
\item
  \texttt{int\ tmu\_opt\_offset}: set the optimized clock offset of GPU.
\item
  \texttt{adj\_gpu(device,\ tmu\_base\_freq,\ 338000)}: set the power
  limit of GPU.
\item
  \texttt{int\ pd\_curr\_freq} and \texttt{int\ pd\_base\_freq}: set the
  current and based clock frequency of CPU. They should be the same.
\item
  \texttt{bool\ reclaim\_slack}: control if we want to enable Slack
  Reclamation (BSR or SR).
\item
  \texttt{double\ reclamation\_ratio}: control how much of the slack
  is reclaimed by the task on the critical path.
\item
  \texttt{bool\ overclock}: control if we want to overclock with
  undervolting.
\item
  \texttt{bool\ autoboost}: control if we want to enable hardware R2H.
\item
  \texttt{bool\ COL\_FT} and \texttt{bool\ ROW\_FT} control if we want
  to enable ABFT (single-side or full checksum)
\end{itemize}

\noindent
2. Once the PowerLA framework is built, the MAGMA testing
binary executables can be used to run each matrix decomposition with a
specified input matrix size. The executables can be run with:

\texttt{<build dir>/testing/testing\_*\_gpu -N <size>}

\noindent
3. Configuring the variables for different modes

\begin{tabular}[]{@{}lllll@{}}
\toprule
& Original & R2H & SR & BSR \\ \hline
\texttt{reclaim\_slack} & false & false & true & true \\
\texttt{reclaimnation\_ratio} & N/A & N/A & 0 & 0-1 \\
\texttt{overclock} & false & false & false & true \\
\texttt{autoboost} & false & true & false & false \\
\texttt{COL\_FT/ROW\_FT} & false & false & false & true \\ \hline
\end{tabular}

\noindent
4. When each test finishes execution it will output:

\begin{itemize}
\item
  Energy consumption of CPU and GPU (total)
\item
  Time cost (per operation \& total)
\item
  Predicted time cost (per iteration)
\item
  The slack prediction error (total average)
\item
  Clock frequency of CPU and GPU (per iteration)
\item
  Decisions on slack reclamation (per iteration)
\end{itemize}
